# Supplementary material for: AutoLink: Self-supervised Learning of Human Skeletons and Object Outlines by Linking Keypoints
Source: arXiv:2205.10636 source file (2023-03-23)
Supplement: Supplementary file 1 [file supp_ablation.tex]

% \section{General Ablation Tests} \label{supp:ablation}

% \hr{[Moved from main document]}In this section, we analyze the hyperparameters and demonstrate the robustness of our model. We also discuss the possible variants of our model and show the superiority of our design. 

% \begin{figure}
% \floatbox[{\capbeside\thisfloatsetup{capbesideposition={right,top},capbesidewidth=0.23\textwidth}}]{figure}[\FBwidth]
% {\caption{\textbf{Examples of different numbers of detected keypoints.} With very few keypoints, the model only models a very basic shape, such as the box on the face, and sometimes cannot fully capture the structure. For example, with K=4, only legs are modeled on humans. With abundant keypoints, it is able to model details.}}
% {\includegraphics[width=0.75\textwidth]{images/ablation_n_kp.jpg}}
% \label{fig:ablation_kp}
% \end{figure}

% \parag{Number of Keypoints \& Thickness}. 
% We show ablation test results on the different numbers of keypoints and edge thicknesses in Figure~\ref{fig:ablation_kp_thick}. The exact numbers can be found in Table~\ref{tab:hyper} in Appendix~\ref{supp:ablation_test}. Our model shows very strong robustness to edge thickness. The accuracy remains state-of-the-art while the thickness of the edges varies by multiple orders of magnitude.
% On the other hand, with the increasing number of keypoints the accuracy increases. This is expected since more keypoints are able to capture structure in more detail, as shown in Figure~\ref{fig:ablation_kp}. 

% \parag{Masking Strategy}. 
% In our standard setting, the image is divided into $16\times 16$ patches and 80\% of the patches are randomly masked. We investigate how the patch size and masking ratio affect the model performance. Figure~\ref{fig:ablation_masking} shows that a too low masking ratio enables the network to directly infer the structure from the masked image which is undesired in our case.
% %the masking ratio cannot be small, because otherwise the structure can be directly inferred from the masked image. 
% In these cases, the network would not choose to infer a set of compact keypoints from the original image. Figure~\ref{fig:ablation_masking} illustrates that the patch size cannot be too small ($4\times 4$) or too large ($64\times 64$). Although in some cases, such as CelebA-in-the-Wild, a different masking strategy gives better results (4.14 vs 5.24), we choose to report a unified strategy that we mask 80\% of $16\times16$ patches for simplicity and conciseness.

% \begin{table}[t]
% \centering
% \caption{\textbf{Ablation tests on variants of edge heatmap generation}. The original design is proved to be the most robust one. Although in some cases it is not optimal, the difference is almost trivial.}
% \resizebox{0.9\linewidth}{!}{%
% \begin{tabular}{lcccc}
% \Xhline{1.5pt}
% Model & CelebA in The Wild $\downarrow$ & Human3.6m $\downarrow$ & DeepFashion $\uparrow$ & Taichi $\downarrow$\\ \Xhline{1.5pt}
% original model & \textbf{5.24}\%  & \textbf{2.76}\% & 65.8\% & 316 \\ 
% fixed $\alpha$ & 6.39\%  & 2.87\% & \textbf{66.0}\% & 374 \\
% shared learnable thickness & 6.12\%  & 3.25\% & 49.1\% & 425 \\
% independent learnable thickness & 5.94\%  & 3.73\% & 50.2\% & \textbf{311} \\
% edge-specific heatmap & 5.65\%  & 3.83\% & 65.1\% & 407\\
% only using keypoints without edges & 6.55\% & 3.58\% & 52.9\% & 722\\
% \Xhline{1.5pt}
% \end{tabular}
% }
% \label{tab:ablation_edge_gen}
% \end{table}

% % \begin{figure}[t]
% % \begin{center}
% %   \includegraphics[width=1.\textwidth]{images/ablation_edge.pdf}
% % \end{center}
% %    \caption{(a) If we do not model the edges, the model may degenerate. (b) If we give different edges a different channel in the feature map, the model would give dummy edges. (c) If the model is trained on the dataset with structured background, the background would be modeled. However, the keypoints can be separated into two sets by spectral clustering. (d) failure case: left) the model cannot model the occlusion well; right) the model has left and right ambiguity.}
% % \label{fig:ablation_edge}
% % \end{figure}

% \parag{Variants of Edge Heatmap Generation}. 
% Besides the heatmap generation described in Method~\ref{sec:method}, we test four more ways to generate the edge maps: 1) we define the thickness as a globally learnable parameter; 2) we learn each edge thickness independently as a learnable parameter; 3) we treat each edge heatmap as an independent channel of the feature map, instead of making them a single channel heatmap with Equation~\ref{eq:max_heatmap}; 4) instead of using the edge heatmap, we generate Gaussian heatmaps for the keypoints and use Equation~\ref{eq:max_heatmap} to combine them in a single channel heatmap. The results are listed in Table~\ref{tab:ablation_edge_gen}. Overall, these variants have worse performance. Although in some cases, the model has slightly better results on specific datasets, the performance boost does not hold in general. We observe that with only keypoints without edges, the model may degenerate, as shown in Figure~\ref{fig:ablation_edge}a. Interestingly, assigning each edge a different channel performs worse than simply combining all edges into a single channel. We believe it is caused by entangling the edge weights with the convolution kernel weights. As visualized in Figure~\ref{fig:ablation_edge}b, there exist dummy edges that do not model the object structure.
% In addition, we tried to remove the learnable $\alpha$ in Equation~\ref{eq:recon}, fixing $\alpha=1$, but the overall performance decreases as shown in Table~\ref{tab:ablation_edge_gen}.

% \parag{Does Texture Matter?} 
% \md{We trained two networks on the horses and zebra separately.} As shown in Figure~\ref{fig:teaser}a, the horse and the zebra share similar shape structures but only one is textured. The striped texture not having a significant impact on the learned structure shows that our model primarily learns the structure instead of texture features.

% \parag{What if the model is trained on the structured background?} We tested on Human3.6m with background, where all images are taken in a single room. The error is 5.02. As shown in Figure~\ref{fig:ablation_edge}c, our model captures the entrance in the background. It is expected since we assume the foreground object is structured. If we apply spectral clustering \cite{ng2001spectral} on the learned graph, the keypoints are clearly divided into two clusters.
